# Supplementary material for: Numerically computing the index of mean curvature flow self-shrinkers
Source: arXiv:2007.06094 ancillary file (2020-07-12)

```
In [1]: # Yakov Berchenko-Kogan
# Code accompanying "Numerically Computing the Index of
# Mean Curvature Flow Self-Shrinkers"
```

```
In [2]: import sympy as sy
import numpy as np
import scipy as sc
import matplotlib.pyplot as plt

sy.init_printing()
plt.rc('text', usetex=True)
plt.rc('font', family='serif', size=11)
plt.rcParams['text.latex.preamble']=[r'\usepackage{amsmath}']
```

```
In [3]: # Load the previously computed cross-section of the Angenent torus
# with 2048 points.
curve = np.load('angenent2048.npy')
M = len(curve)
plt.plot(*curve.T)
```

```
Out[3]: [<matplotlib.lines.Line2D at 0x7f8f85506630>]
```

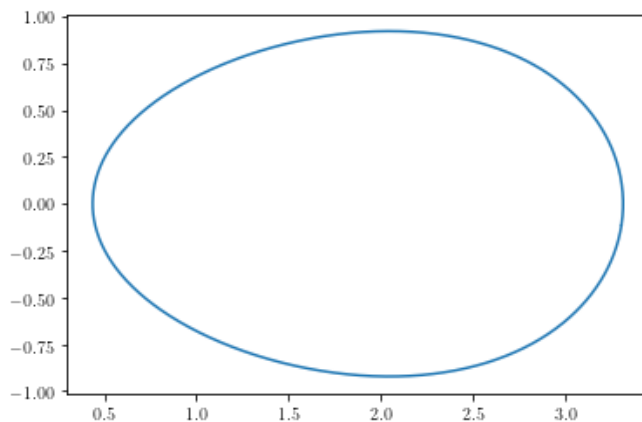

```
In [4]: kmax = 4 # We will compute  $L_k$  for  $k < kmax$ .
```

```
In [5]: # Symbolically compute the discrete distance and its Hessian.
r, z, r1, z1, r2, z2 = sy.symbols('r z r1 z1 r2 z2')

conformalFactor = r / 2 * sy.exp(-(r**2 + z**2)/4)

# Evaluate the conformal factor at the midpoint and
# multiply by the Euclidean distance.
discreteDistanceSymbolic = conformalFactor.subs(
    [(r, (r1+r2)/2), (z, (z1+z2)/2)]
) * sy.sqrt((r2-r1)**2 + (z2-z1)**2)

# Compute the Hessian of the discrete distance.
hessSymbolic = sy.hessian(discreteDistanceSymbolic, (r1, z1, r2, z2))

# Create fast functions to compute the symbolic expressions.
discreteDistance = sy.lambdify((r1, z1, r2, z2), discreteDistanceSymbolic)
hess = sy.lambdify((r1, z1, r2, z2), hessSymbolic)

discreteDistanceSymbolic
```

Out[5]:

$$\frac{\left(\frac{r_1}{2} + \frac{r_2}{2}\right) \sqrt{(-r_1 + r_2)^2 + (-z_1 + z_2)^2} e^{-\frac{\left(\frac{r_1}{2} + \frac{r_2}{2}\right)^2}{4} - \frac{\left(\frac{z_1}{2} + \frac{z_2}{2}\right)^2}{4}}}{2}$$

```
In [6]: # Compute the length of the cross-section with respect to the weighted metric.
# This length is the entropy of the Angenent torus.
length = 0
for m in range(M) :
    length += discreteDistance(*curve[m-1], *curve[m])
length
```

Out[6]: 1.8512185857915548

```
In [7]: %%time
# hessians[m] is the Hessian of the discrete distance, evaluated at
# (q_m, q_{m+1}). This quantity is denoted H_{m, m+1} in the paper.
hessians = np.empty((M, 4, 4))
for m in range(M) :
    hessians[m] = hess(*curve[m], *curve[(m+1) % M])
```

CPU times: user 1.63 s, sys: 9.72 ms, total: 1.64 s  
Wall time: 1.61 s

```
In [8]: # normals[m] is the normal vector to the curve at q_m.
# This quantity is denoted \mathbf{n}_m in the paper.
normals = np.empty((M, 2))
for m in range(M) :
    Hm = hessians[m-1, 2:, 2:] + hessians[m, :2, :2] # The matrix H_m.
    _, vs = np.linalg.eigh(Hm)
    normals[m] = vs[1]

#Ensure outward pointing normals.
tangent = curve[(m+1) % M] - curve[m-1]
if np.cross(normals[m], tangent) < 0:
    normals[m] *= -1
```

```
In [9]: # L0 is -L_{0; d} in the paper.
L0 = np.zeros((M,M))
for m in range(M) :
    # NT is \mathbf{N}_{m, m+1}^T in the paper.
    NT = sc.linalg.block_diag(normals[m], normals[(m+1) % M])
    # L0m is -L_{0; m, m+1} in the paper.
    L0m = M / length * NT.dot(hessians[m]).dot(NT.T)
    for i in range(2) :
        for j in range(2) :
            L0[(m+i) % M, (m+j) % M] += L0m[i, j]
```

```
In [10]: # Lks[k] is -L_{k; d} in the paper.
Lks = np.empty((kmax, M, M))
# Rn2 is the diagonal matrix with entries r_m^{-2}, denoted R_d^{-2} in the paper.
Rn2 = np.diag(curve[:, 0]**(-2))
for k in range(kmax) :
    Lks[k] = L0 + k**2 * Rn2 # L0 + k^2/r^2
```

```
In [11]: %%time
# eks[k] and uks[k] are the eigenvalues and eigenvectors of -L_{k; d}.
eks = np.empty((kmax, M))
uks = np.empty((kmax, M, M))
for k in range(kmax) :
    eks[k], uks[k] = np.linalg.eigh(Lks[k])
```

CPU times: user 12.6 s, sys: 211 ms, total: 12.8 s  
Wall time: 2.14 s

```

In [12]: def plotCurveVariation(k, j) :
    variation = uks[k, :, j] #  $u_m$ .
    normalVariation = variation[:, np.newaxis] * normals #  $u_m \mathbf{\hat{n}}_m$ .
    # Scaling factor for the eigenvectors so the plots look nice.
    variationScaling = -.05 * np.sqrt(M)

    plt.plot(*curve.T)
    plt.plot(*(curve + variationScaling * normalVariation).T, '--')
    plt.title('$k={}$, $\lambda={:f}$'.format(k, eks[k, j]))
    plt.xlabel('$r$')
    plt.ylabel('$z$')
    plt.gca().set_aspect('equal', 'box')
    plt.xlim((0, 4))
    plt.ylim((-1.3, 1.3))

    for k in range(kmax) :
        for j in range(M) :
            if eks[k, j] < 0 :
                plotCurveVariation(k, j)
                plt.show()

```

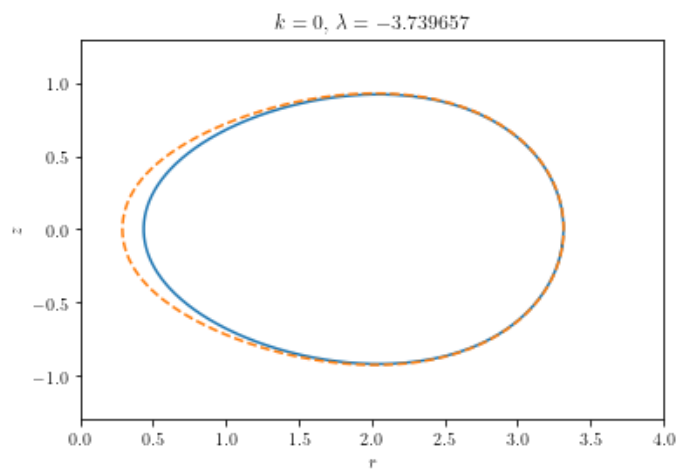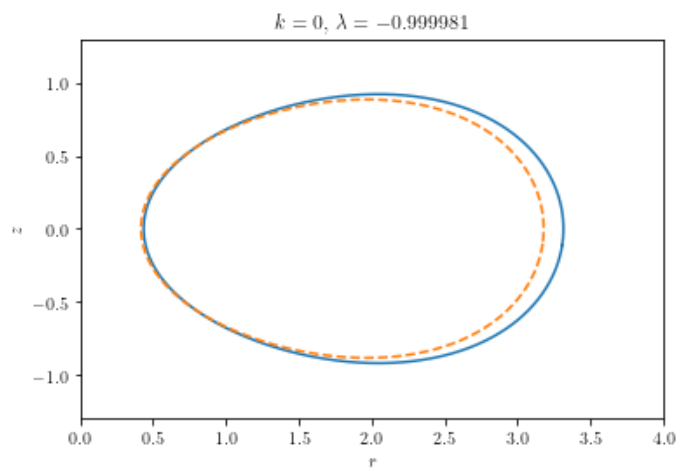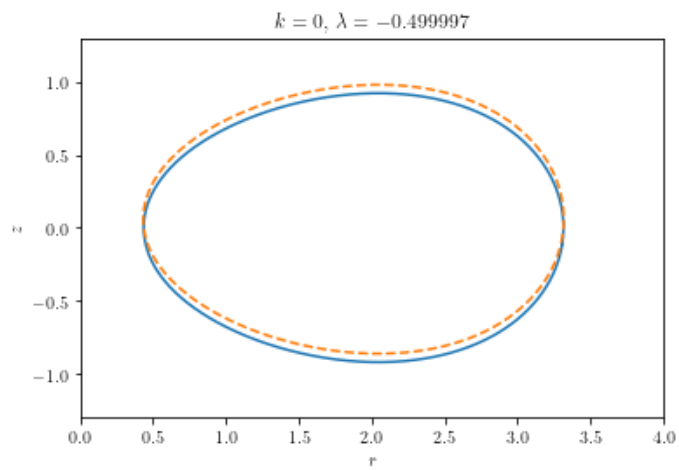

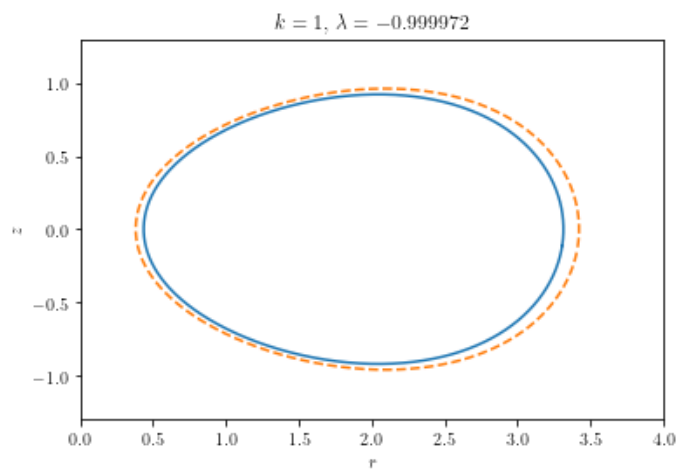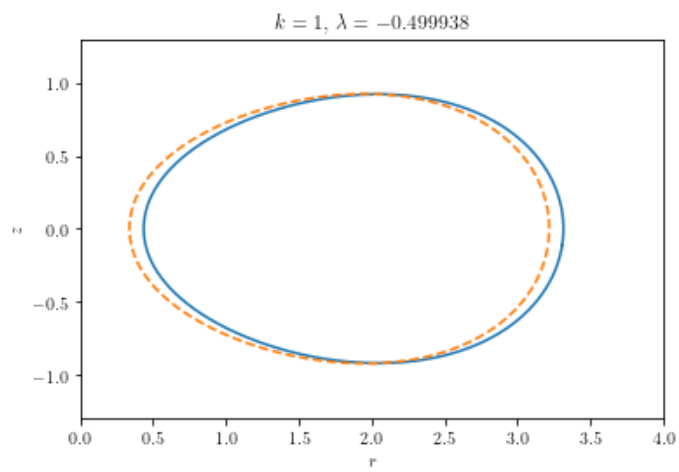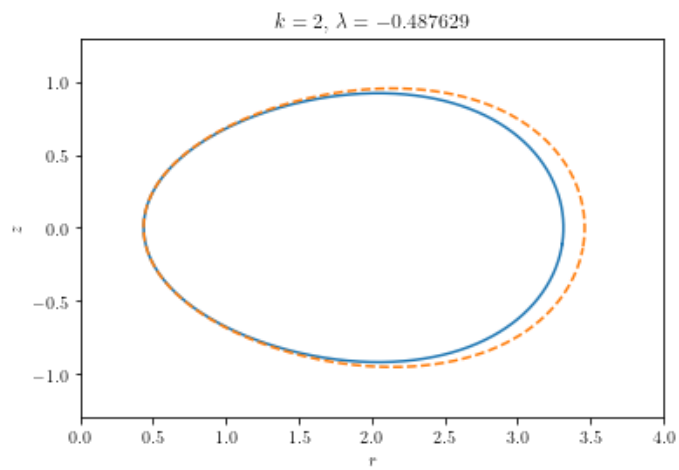

Supplement: Supplementary file 1 [file AngenentIndex.pdf]
